# Supplementary material for: DyAdHyTM: A Low Overhead Dynamically Adaptive Hybrid Transactional Memory on Big Data Graphs
Source: arXiv:1702.07081 source file (2017-03-02)
Supplement: Supplementary file 1 [file appendix.tex]

%\newpage
\section{Appendix}\label{Sec:appendix}
In this appendix, we are putting our figures in bigger size so that it is easier for the reviewers to see the details that might not appear as clearly in the middle of the paper. Figures shows thread counts lower than 4 for all the figures in the paper. We show only thread counts starting at 4 in the paper for better readability.
%First six figures are Figures~\ref{fig:data3}(\subref{fig:fig1}) through (\subref{fig:fig6}).
%\vspace{-5in}
\begin{figure*}[b]
\centering
%\minipage{0.32\textwidth}
%  \begin{subfigure}{\linewidth}
  \includegraphics[width={\linewidth}]{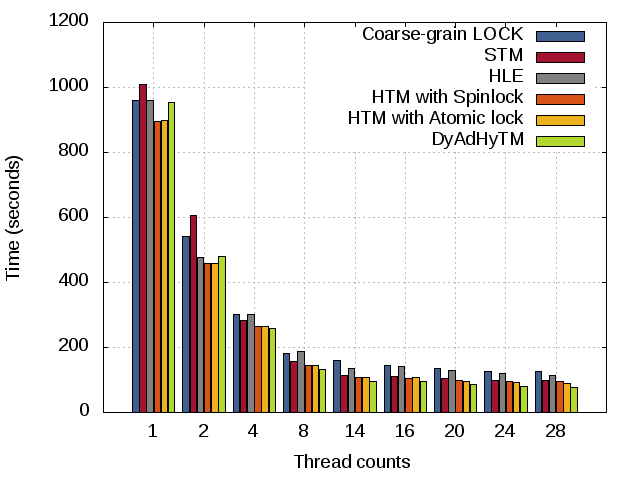}
  %\caption{Two kernels}\label{fig:dataTotal_s26}
  \caption{Performance of the combined Generate and Compute Kernels with DyAdHyTM  compared to coarse grain lock, STM, HLE, HTM with Spinlock and Atomic lock for scale 26 on a 28-core SMP node with 64 GBs memory, x-axis represents thread counts, y-axis represents execution time in seconds. This is a scaled up repeat of Figure~\ref{fig:data3}(\subref{fig:fig1})}
%  \end{subfigure}%
\end{figure*}
%\endminipage\hfill
%\minipage{0.32\textwidth}
\begin{figure*}
%  \begin{subfigure}{\linewidth}
  \includegraphics[width=\linewidth]{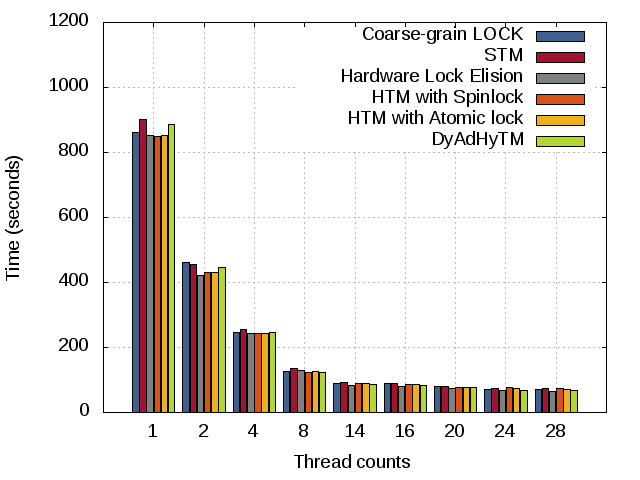}
  %\caption{Generation Kernel}\label{fig:data_s26_Gen}
%  \caption{Scale 26: Generate \label{fig:fig2}}
  \caption{Performance of the Generate Kernel with DyAdHyTM compared to coarse grain lock, STM, HLE, HTM with Spinlock and Atomic lock for  scale 26 on a 28-core SMP node with 64 GBs memory, x-axis represents thread counts, y-axis represents execution time in seconds. This is a scaled up repeat of Figure~\ref{fig:data3}(\subref{fig:fig2})}

%  \end{subfigure}%
\end{figure*}
%\endminipage\hfill
%\minipage{0.32\textwidth}%
\begin{figure*}
%\begin{subfigure}{\linewidth}
  \includegraphics[width=\linewidth]{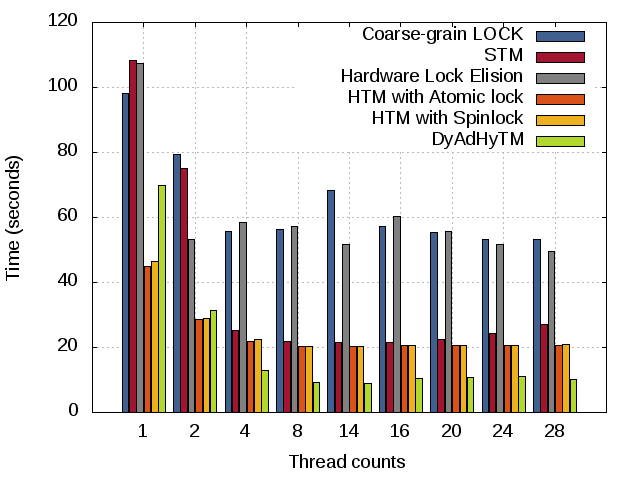}
  %\caption{Computation Kernel}\label{fig:data_s26_CK}
%  \caption{Scale 26: Compute\label{fig:fig3}}
  \caption{Performance of the Compute Kernel with DyAdHyTM  compared to coarse grain lock, STM, HLE, HTM with Spinlock and Atomic lock for  scale 26 on a 28-core SMP node with 64 GBs memory, x-axis represents thread counts, y-axis represents execution time in seconds.
This is a scaled up repeat of Figure~\ref{fig:data3}(\subref{fig:fig3})}
  
%  \end{subfigure}%
\end{figure*}
%\minipage{0.32\textwidth}
  %\hfill
\begin{figure*}
%  \begin{subfigure}{\linewidth}
  \includegraphics[width=\linewidth]{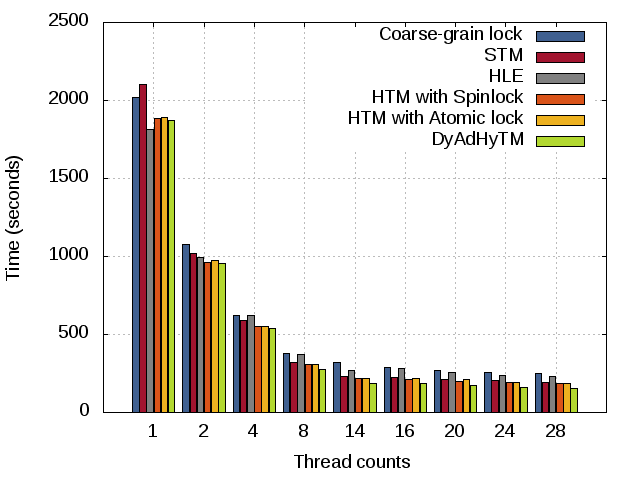}
  %\caption{Two kernels}\label{fig:dataTotal_s26}
 % \caption{Scale 26: Two Kernel\label{fig:fig4}}
  \caption{Performance of the combined Generate and Compute Kernels with DyAdHyTM  compared to coarse grain lock, STM, HLE, HTM with Spinlock and Atomic lock for large scale 27 on a 28-core SMP node with 64 GBs memory, x-axis represents thread counts, y-axis represents execution time in seconds.
This is a scaled up repeat of Figure~\ref{fig:data3}(\subref{fig:fig4})}
%  \end{subfigure}%
\end{figure*}
%\endminipage\hfill
%\minipage{0.32\textwidth}
\begin{figure*}
%  \begin{subfigure}{\linewidth}
  \includegraphics[width=\linewidth]{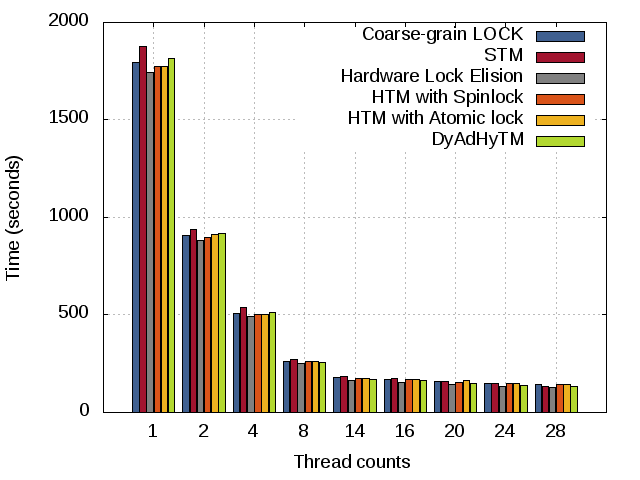}
  %\caption{Generation Kernel}\label{fig:data_s26_Gen}
%  \caption{Scale 27: Generate\label{fig:fig5}}
  \caption{Performance of the Generate Kernel with DyAdHyTM compared to coarse grain lock, STM, HLE, HTM with Spinlock and Atomic lock for  scale 27 on a 28-core SMP node with 64 GBs memory, x-axis represents thread counts, y-axis represents execution time in seconds. This is a scaled up repeat of Figure~\ref{fig:data3}(\subref{fig:fig5}.}

%\end{subfigure}%
\end{figure*}
%\endminipage\hfill
%\minipage{0.32\textwidth}%
\begin{figure*}
%  \begin{subfigure}{\linewidth}
  \includegraphics[width=\linewidth]{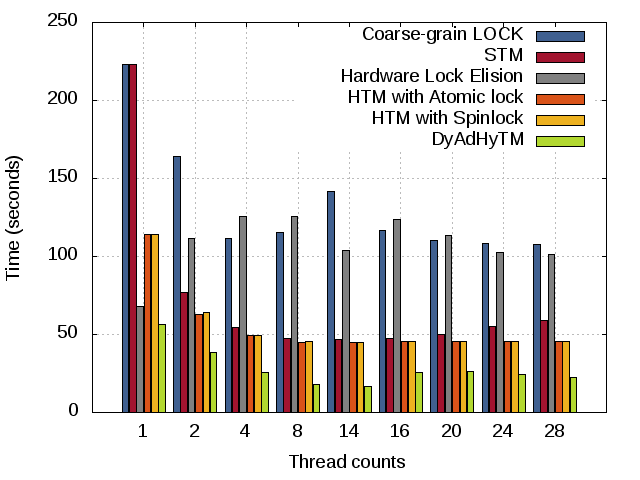}
  %\caption{Computation Kernel}\label{fig:data_s26_CK}
%  \caption{Scale 27: Compute\label{fig:fig6}}
  \caption{Performance of the Compute Kernel with DyAdHyTM  compared to coarse grain lock, STM, HLE, HTM with Spinlock and Atomic lock for  scale 27 on a 28-core SMP node with 64 GBs memory, x-axis represents thread counts, y-axis represents execution time in seconds.
This is a scaled up repeat of Figure~\ref{fig:data3}(\subref{fig:fig6}).}
%\end{subfigure}%
\end{figure*}
%\endminipage
%\caption{Performance improvement for 2 kernels (\subref{fig:fig1}) and (\subref{fig:fig4}), generation kernel (\subref{fig:fig2}) and (\subref{fig:fig5}), computation kernel (\subref{fig:fig3}) and (\subref{fig:fig6}) with AdHyTM  over coarse grain lock, STM, HLE, HTM for large scale 26 and 27 on a 28-core SMP node with 64 GBs memory, x-axis represents thread counts, y-axis represents execution time in seconds}
%\label{fig:data3}
%\end{figure*}

\begin{figure*}
%  \begin{subfigure}{\linewidth}
  \includegraphics[width=\linewidth]{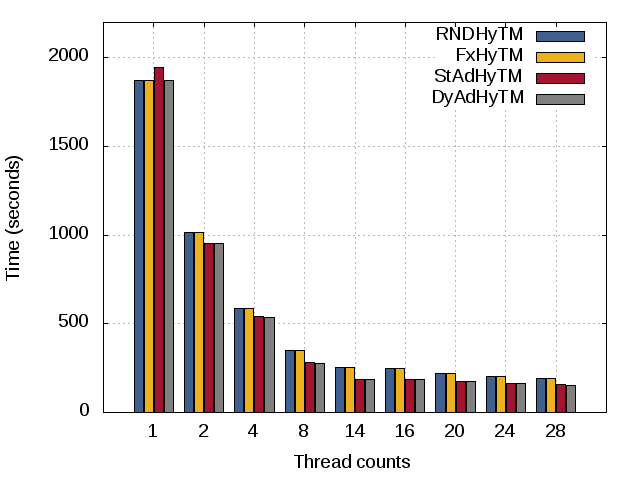}
  %\caption{Two kernels}\label{fig:dataTotal_s26}
 % \caption{Scale 26: Two Kernel\label{fig:fig4}}
  \caption{Performance of the combined Generate and Compute Kernels with DyAdHyTM compared to RNDHyTM, FxHyTM, StAdHyTM for scale 27 on a 28-core SMP node with 64 GBs memory, x-axis represents thread counts, y-axis represents execution time in seconds.
This is a scaled up repeat of Figure~\ref{fig:data3}(\subref{fig:fig4})}
%  \end{subfigure}%

\end{figure*}
%\endminipage\hfill
%\minipage{0.32\textwidth}
\begin{figure*}
%  \begin{subfigure}{\linewidth}
  \includegraphics[width=\linewidth]{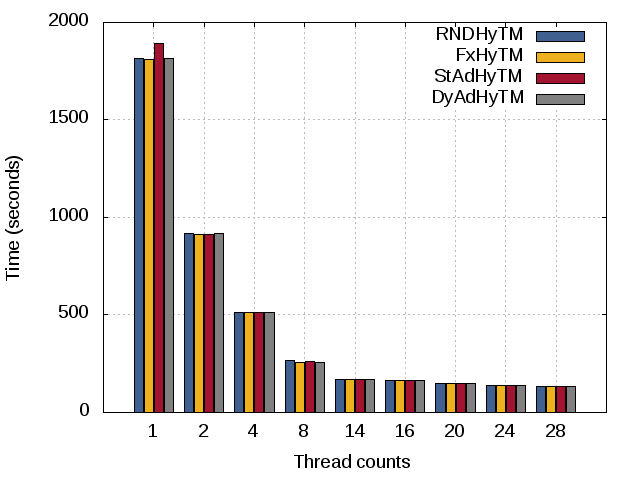}
  %\caption{Generation Kernel}\label{fig:data_s26_Gen}
%  \caption{Scale 27: Generate\label{fig:fig5}}
  \caption{Performance of the Generate Kernel with DyAdHyTM compared to RNDHyTM, FxHyTM, StAdHyTM scale 27 on a 28-core SMP node with 64 GBs memory, x-axis represents thread counts, y-axis represents execution time in seconds. This is a scaled up repeat of Figure~\ref{fig:data3}(\subref{fig:fig5}.}

%\end{subfigure}%
\end{figure*}
%\endminipage\hfill
%\minipage{0.32\textwidth}%
\begin{figure*}
%  \begin{subfigure}{\linewidth}
  \includegraphics[width=\linewidth]{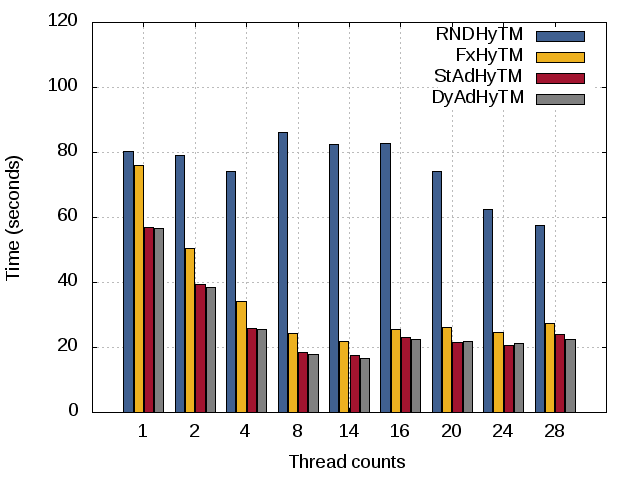}
  %\caption{Computation Kernel}\label{fig:data_s26_CK}
%  \caption{Scale 27: Compute\label{fig:fig6}}
  \caption{Performance of the Compute Kernel with DyAdHyTM compared to RNDHyTM, FxHyTM, StAdHyTM for scale 27 on a 28-core SMP node with 64 GBs memory, x-axis represents thread counts, y-axis represents execution time in seconds.
This is a scaled up repeat of Figure~\ref{fig:data3}(\subref{fig:fig6}).}
%\end{subfigure}%
\end{figure*}
%\endminipage
%\caption{Performance improvement for 2 kernels (\subref{fig:fig1}) and (\subref{fig:fig4}), generation kernel (\subref{fig:fig2}) and (\subref{fig:fig5}), computation kernel (\subref{fig:fig3}) and (\subref{fig:fig6}) with AdHyTM  over coarse grain lock, STM, HLE, HTM for large scale 26 and 27 on a 28-core SMP node with 64 GBs memory, x-axis represents thread counts, y-axis represents execution time in seconds}
%\label{fig:data3}
%\end{figure*}

\begin{figure*}
\centering
%\minipage{0.32\textwidth}
%  \begin{subfigure}[b]{0.9\linewidth}
  \includegraphics[width=\linewidth]{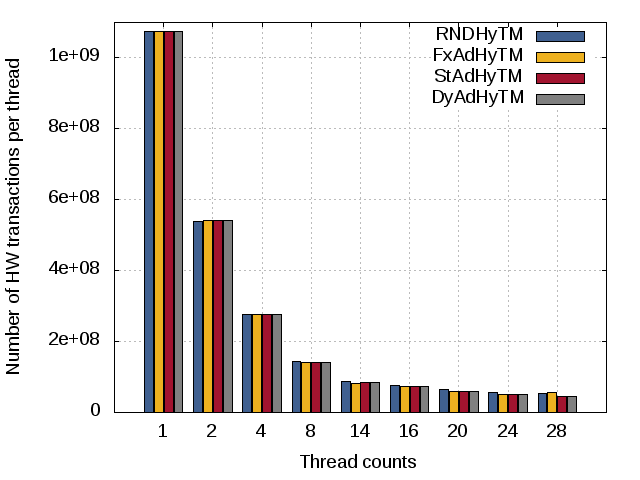}
  %\caption{Two kernels}\label{fig:dataTotal_s26}
  %\caption{Scale 27: HTM transactions\label{fig:fig13}}
  \caption{Number of HTM transactions for per thread for scale 27 for RNDHyTM, FxHyTM, StAdHyTM, and DyAdHyTM on a 28-cores SMP node with 64 GBs memory}
\label{fig:data4X1}
\end{figure*}
\begin{figure*}
  %\begin{subfigure}[b]{0.9\linewidth}
  \includegraphics[width=\linewidth]{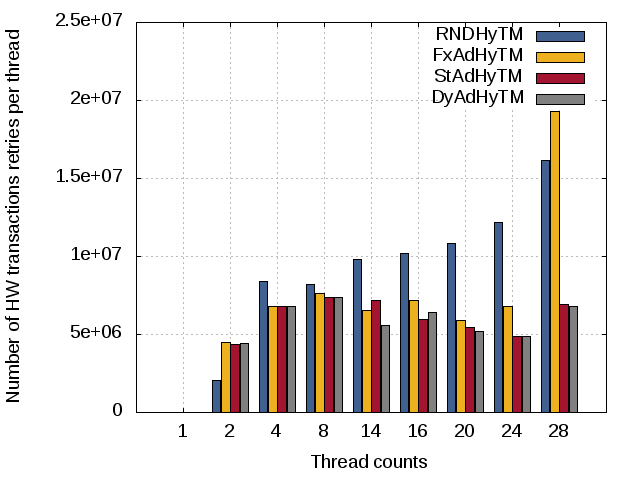}
  %\caption{Two kernels}\label{fig:dataTotal_s26}
  %\caption{Scale 27: Retries\label{fig:fig23}}
  \caption{Number of HW Transaction Retries per thread for RNDHyTM, FxHyTM, StAdHyTM, and DyAdHyTM for scale 27 on a 28-cores SMP node with 64 GBs memory}
  %\end{subfigure}%
  \end{figure*}
%\endminipage\hfill
%\minipage{0.32\textwidth}
\begin{figure*}
  %\begin{subfigure}[b]{0.9\linewidth}
  \includegraphics[width=\linewidth]{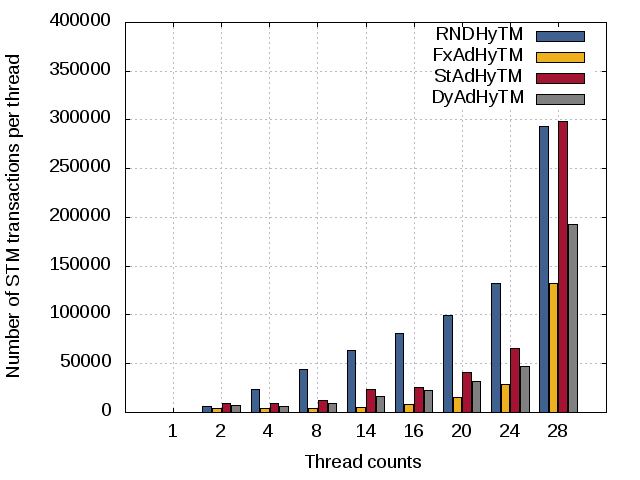}
  %\caption{Generation Kernel}\label{fig:data_s26_Gen}
  %\caption{Scale 27: STM fallbacks\label{fig:fig33}}
  %\end{subfigure}%
%\endminipage
\caption{Number of STM transactions per thread for RNDHyTM, FxHyTM, StAdHyTM, and DyAdHyTM for  scale 27 on a 28-cores SMP node with 64 GBs memory}
\label{fig:data4X2}
\end{figure*}

\begin{figure}
\lstset{language=C}  
% Set your language (you can change the language for each code-block optionally)
% Start your code-block
\begin{lstlisting}[frame=single]
tries= NUM_RETRIES
if HW_BEGIN begins successfully
  if (gbllock is locked) 
    abort
  else
    transactional code
    HW_COMMIT
else if (tries >= 0)
  decrement tries 
  retries in HW
else //retrials quota ends
  //execution in lock
  while wait for lock to be free
  	atomic add(gblloc ,1)
  	transactional code
  	atomic sub(gblloc ,1)
return 
\end{lstlisting}
\caption{Hardware Transactional Memory with Atomic Lock Pseudo Code}
\label{fig:HTMAlock}
\end{figure}

\begin{figure}
\lstset{language=C}  
% Set your language (you can change the language for each code-block optionally)
% Start your code-block
\begin{lstlisting}[frame=single]
tries= NUM_RETRIES
if HW_BEGIN begins successfully
  if (gbl_spinlock locked)
    abort
  else
    transactional code
    HW_COMMIT
else if (tries >= 0)
  decrement tries 
  retries in HW
else //retrials quota ends
  //execution in lock
  while wait for lock to be free
  	lock gbl_spinlock
  	transactional code
  	unlock gbl_spinlock
return 
\end{lstlisting}
\caption{Hardware Transactional Memory with Spin Lock Pseudo Code}
\label{fig:HTMSlock}
\end{figure}
